# Supplementary material for: DublinCity: Annotated LiDAR Point Cloud and its Applications
Source: arXiv:1909.03613 source file (2019-09-06)
Supplement: Supplementary file 1 [file suppl_mat_3Dreconst-SR.tex]

\subsection*{Image-based 3D reconstruction evaluation}
%\subsubsection*{Aerial imagery description}
%The LiDAR point cloud acquisition was the primary output of the aerial scanning. However, the helicopter also collected imagery during the flight~\cite{laefer20172015}. In this supplementary material, the two sets of images used in the paper are detailed.

%\textbf{Top view imagery}.\label{subsec:GeoRegisteredRGB} The dataset includes 4471 images taken from a helicopter an are called in the cited repository as Geo-referenced RGB. The resolution in pixels of the images is $9000\times6732$ and are stored in TIFF format, with a ground sampling distance of 3.4 cm. The total size of the images is 813 GB and they are presented in the different flight paths. The geographic information is given as GPS tag in the EXIF metadata and the camera used for the capture is Leica RCD30. 

%\textbf{Oblique view imagery}.\label{subsec:ObliqueImagery} The oblique imagery contains 4033 JPEG images which are taken with two different NIKON D800E cameras. They are referred to as Oblique photos, their resolution is $7360\times4912$ and its size is 18.5 GB. As it happens with geo-registered RGB images, they are presented in accordance with the flight path but including an extra subdivision which corresponds to each camera.

\subsubsection*{Additional figures}
\begin{figure}[!h]
    \centering
    %[width=0.35\linewidth] [width=0.50\linewidth]
    \includegraphics[width=0.48\linewidth]{figures/3dRecons/suppl_mat/oblique_tiles.png}
    \includegraphics[width=0.48\linewidth]{figures/3dRecons/suppl_mat/rgb_tiles.png}
    \caption{Image-based reconstruction in the overlapping area. On the left, the result with the oblique view imagery; on the right, with the top view imagery}
    \label{fig:3dRecons:suppl_mat}
\end{figure}
\begin{figure}[!h]
    \centering
    %[width=0.35\linewidth] [width=0.50\linewidth]
    \includegraphics[width=0.24\linewidth]{figures/3dRecons/suppl_mat/ICP_registration/before_ICP_oblique_detail.png}
    \includegraphics[width=0.24\linewidth]{figures/3dRecons/suppl_mat/ICP_registration/before_ICP_oblique_2_detail.png}
    \includegraphics[width=0.24\linewidth]{figures/3dRecons/suppl_mat/ICP_registration/before_ICP_RGB_detail.png}
    \includegraphics[width=0.24\linewidth]{figures/3dRecons/suppl_mat/ICP_registration/before_ICP_RGB_2_detail.png}
    \\
    \includegraphics[width=0.24\linewidth]{figures/3dRecons/suppl_mat/ICP_registration/after_ICP_oblique_detail.png}
    \includegraphics[width=0.24\linewidth]{figures/3dRecons/suppl_mat/ICP_registration/after_ICP_oblique_2_detail.png}
    \includegraphics[width=0.24\linewidth]{figures/3dRecons/suppl_mat/ICP_registration/after_ICP_RGB_detail.png}
    \includegraphics[width=0.24\linewidth]{figures/3dRecons/suppl_mat/ICP_registration/after_ICP_RGB_2_detail.png}
    \caption{Top row shows some details of the reconstruction with the coarse registration done with the GPS data. Second row, shows the same details after ICP registration. LiDAR point cloud, reconstruction with oblique images and reconstruction with top view images are shown in yellow, cyan and blue, respectively. }
    \label{fig:3dRecons:suppl_mat:ICP_registration}
\end{figure}
